# Supplementary material for: Nonperturbative running of the tensor operator for $N_\rm{f}=3$ QCD from the chirally rotated Schr\"odinger Functional
Source: arXiv:2311.15046 source file (2023-11-25)
Supplement: Supplementary file 2 [file appendixC.tex]

\section{Continuum extrapolation results from the $\sigmaT$:$u$-by-$u$ and $\gammaT$:$u$-by-$u$ methods} 
\label{app:sigma-rho-he}

\providecommand{\tabularnewline}{\\}

\begin{table}[h]
{\footnotesize
\begin{tabular}{|c||c|c|c||c|c|c|}
$u$ & $\sigmaT$ & $\rho_{\mathrm T}$ & $\dfrac{\chi^{2}}{\mathrm{d.o.f.}}$ & $\sigmaT^{\mathrm{sub}}$ & $\rho_{\mathrm T}^{\mathrm{sub}}$ & $\dfrac{\chi^{2}}{\mathrm{d.o.f.}}$ \tabularnewline
& & & & & & \tabularnewline
\hline 
1.11 & 1.0206(13) & -0.173(56) & 1.2 & 1.0200(13) & -0.026(56) & 1.65\tabularnewline
1.1844 & 1.0249(13) & -0.374(58) & 0.62 & 1.0242(13) & -0.217(58) & 0.38\tabularnewline
1.2656 & 1.0243(15) & -0.282(66) & 0.13 & 1.0234(15) & -0.113(66) & 0.03\tabularnewline
1.3627 & 1.0310(19) & -0.392(78) & 0.11 & 1.0301(19) & -0.210(79) & 0.04\tabularnewline
1.4808 & 1.0345(16) & -0.426(75) & 0.77 & 1.0335(16) & -0.226(75) & 0.43\tabularnewline
1.6173 & 1.0348(23) & -0.313(96) & 0.62 & 1.0337(23) & -0.093(96) & 0.39\tabularnewline
1.7943 & 1.0434(24) & -0.51(10) & 0.22 & 1.0423(24) & -0.27(11) & 0.1\tabularnewline
2.012 & 1.0540(20) & -0.66(10) & 0.26 & 1.0529(20) & -0.40(10) & 0.14\tabularnewline
\end{tabular}
\caption{Results of the fit parameters $\sigmaT$ and $\rho_{\mathrm T}$ (both non-subtracted and subtracted) in the $\alpha$-scheme.}
\label{tab:sigma-rho-alpha}
}
\end{table}

\begin{table}[h]
{\footnotesize
\begin{tabular}{|c||c|c|c||c|c|c|}
$u$ & $\sigmaT$ & $\rho_{\mathrm T}$ & $\dfrac{\chi^{2}}{\mathrm{d.o.f.}}$ & $\sigmaT^{\mathrm{sub}}$ & $\rho_{\mathrm T}^{\mathrm{sub}}$ & $\dfrac{\chi^{2}}{\mathrm{d.o.f.}}$ \tabularnewline
& & & & & & \tabularnewline
\hline 
1.11 & 1.0187(11) & -0.121(49) & 1.55 & 1.0183(11) & -0.010(50) & 1.91\tabularnewline
1.1844 & 1.0221(11) & -0.282(51) & 0.98 & 1.0217(11) & -0.165(51) & 0.75\tabularnewline
1.2656 & 1.0220(14) & -0.214(60) & 0.13 & 1.0215(14) & -0.087(60) & 0.06\tabularnewline
1.3627 & 1.0270(16) & -0.273(68) & 0.06 & 1.0265(16) & -0.137(68) & 0.02\tabularnewline
1.4808 & 1.0298(13) & -0.299(65) & 0.64 & 1.0292(13) & -0.149(65) & 0.4\tabularnewline
1.6173 & 1.0297(19) & -0.189(81) & 0.26 & 1.0291(19) & -0.026(81) & 0.15\tabularnewline
1.7943 & 1.0371(21) & -0.361(90) & 0.19 & 1.0365(21) & -0.181(90) & 0.11\tabularnewline
2.012 & 1.0448(17) & -0.459(84) & 0.18 & 1.0442(17) & -0.260(85) & 0.13\tabularnewline
\end{tabular}
\caption{Results of the fit parameters $\sigmaT$ and $\rho_{\mathrm T}$ (both non-subtracted and subtracted) in the $\beta$-scheme.}
\label{tab:sigma-rho-beta}
}
\end{table}

\vskip 1.0 cm

\begin{table}[h]
{\footnotesize
\begin{tabular}{|c||c|c|c||c|c|c|}
$u$ & $\sigmaT$ & $\rho_{\mathrm T}$ & $\dfrac{\chi^{2}}{\mathrm{d.o.f.}}$ & $\sigmaT^{\mathrm{sub}}$ & $\rho_{\mathrm T}^{\mathrm{sub}}$ & $\dfrac{\chi^{2}}{\mathrm{d.o.f.}}$ \tabularnewline
& & & & & & \tabularnewline
\hline 
1.11 & 1.01479(89) & -0.238(39) & 0.0 & 1.01387(89) & 0.050(39) & 0.11\tabularnewline
1.1844 & 1.0166(10) & -0.254(45) & 0.06 & 1.0156(10) & 0.054(45) & 0.01\tabularnewline
1.2656 & 1.0190(12) & -0.326(49) & 0.0 & 1.0179(12) & 0.004(49) & 0.11\tabularnewline
1.3627 & 1.0209(13) & -0.368(53) & 0.13 & 1.0198(13) & -0.013(53) & 0.0\tabularnewline
1.4808 & 1.02260(100) & -0.357(48) & 4.28 & 1.02139(100) & 0.027(48) & 2.65\tabularnewline
1.6173 & 1.0252(15) & -0.380(63) & 3.49 & 1.0238(15) & 0.043(63) & 2.39\tabularnewline
1.7943 & 1.0297(16) & -0.519(68) & 1.12 & 1.0284(16) & -0.055(68) & 0.63\tabularnewline
2.012 & 1.0311(13) & -0.359(65) & 0.4 & 1.0297(13) & 0.157(65) & 0.12\tabularnewline
\end{tabular}
\caption{Results of the fit parameters $\sigmaT$ and $\rho_{\mathrm T}$ (both non-subtracted and subtracted) in the $\gamma$-scheme.}
}
\label{tab:sigma-rho-gamma}
\end{table}

\begin{table}
{\footnotesize
\begin{tabular}{|c||c|c|c||c|c|c|}
$u$ & $\sigmaT$ & $\rho_{\mathrm T}$ & $\dfrac{\chi^{2}}{\mathrm{d.o.f.}}$ & $\sigmaT^{\mathrm{sub}}$ & $\rho_{\mathrm T}^{\mathrm{sub}}$ & $\dfrac{\chi^{2}}{\mathrm{d.o.f.}}$ \tabularnewline
& & & & & & \tabularnewline
\hline 
1.11 & 1.01635(71) & 0.065(31) & 0.31 & 1.01664(71) & -0.018(31) & 0.08\tabularnewline
1.1844 & 1.01731(83) & 0.047(36) & 0.24 & 1.01762(83) & -0.041(36) & 0.06\tabularnewline
1.2656 & 1.01768(89) & 0.092(38) & 0.07 & 1.01803(89) & -0.004(38) & 0.28\tabularnewline
1.3627 & 1.01995(100) & 0.101(42) & 0.01 & 1.02028(100) & -0.000(42) & 0.01\tabularnewline
1.4808 & 1.02255(78) & 0.076(38) & 2.4 & 1.02293(78) & -0.034(38) & 1.43\tabularnewline
1.6173 & 1.0249(12) & 0.075(50) & 1.57 & 1.0254(12) & -0.047(50) & 1.03\tabularnewline
1.7943 & 1.0273(12) & 0.173(53) & 1.04 & 1.0277(12) & 0.040(53) & 0.66\tabularnewline
2.012 & 1.03448(97) & 0.020(50) & 0.34 & 1.03491(97) & -0.127(49) & 0.09\tabularnewline
\end{tabular}
\caption{Results of the fit parameters $\sigmaT$ and $\rho_{\mathrm T}$ (both non-subtracted and subtracted) in the $\delta$-scheme.}
\label{tab:sigma-rho-delta}
}
\end{table}

\cleardoublepage
